# Supplementary material for: H\"older Continuity of the Gradient of Solutions to Doubly Non-Linear Parabolic Equations
Source: arXiv:2305.08539 source file (2023-05-15)
Supplement: Supplementary file 1 [file Chapter_Appendix.tex]

%\chapter{Appendix}

\appendix

\
